# Supplementary material for: 3D Feature Prediction for Masked-AutoEncoder-Based Point Cloud Pretraining
Source: arXiv:2304.06911 source file (2024-04-28)
Supplement: Supplementary file 2 [file supp-fig-compare.tex]

\begin{figure*}
    \centering
    \scriptsize
    \begin{overpic}[width=\linewidth]{Images/supp_compare.pdf}
    \put(4,-3.5){Input}
    \put(22,-3.5){GT point normal}
    \put(42,-3.5){Predicted point normal}
    \put(64,-3.5){GT surface variation}
    \put(81,-3.5){Predicted surface variation}
    \end{overpic}
    \vspace{4mm}
    \caption{\textbf{Qualitative results on target features.} The masking ratio of input point cloud is 60\%.} 
    \label{fig:supp-compare} %\vspace{-4mm}
\end{figure*}
