# Supplementary material for: 3D Feature Prediction for Masked-AutoEncoder-Based Point Cloud Pretraining
Source: arXiv:2304.06911 source file (2024-04-28)
Supplement: Supplementary file 3 [file supp-fig-feat-vis-v2.tex]

\begin{figure}[h]
    \centering
    \includegraphics[width=0.7\linewidth]{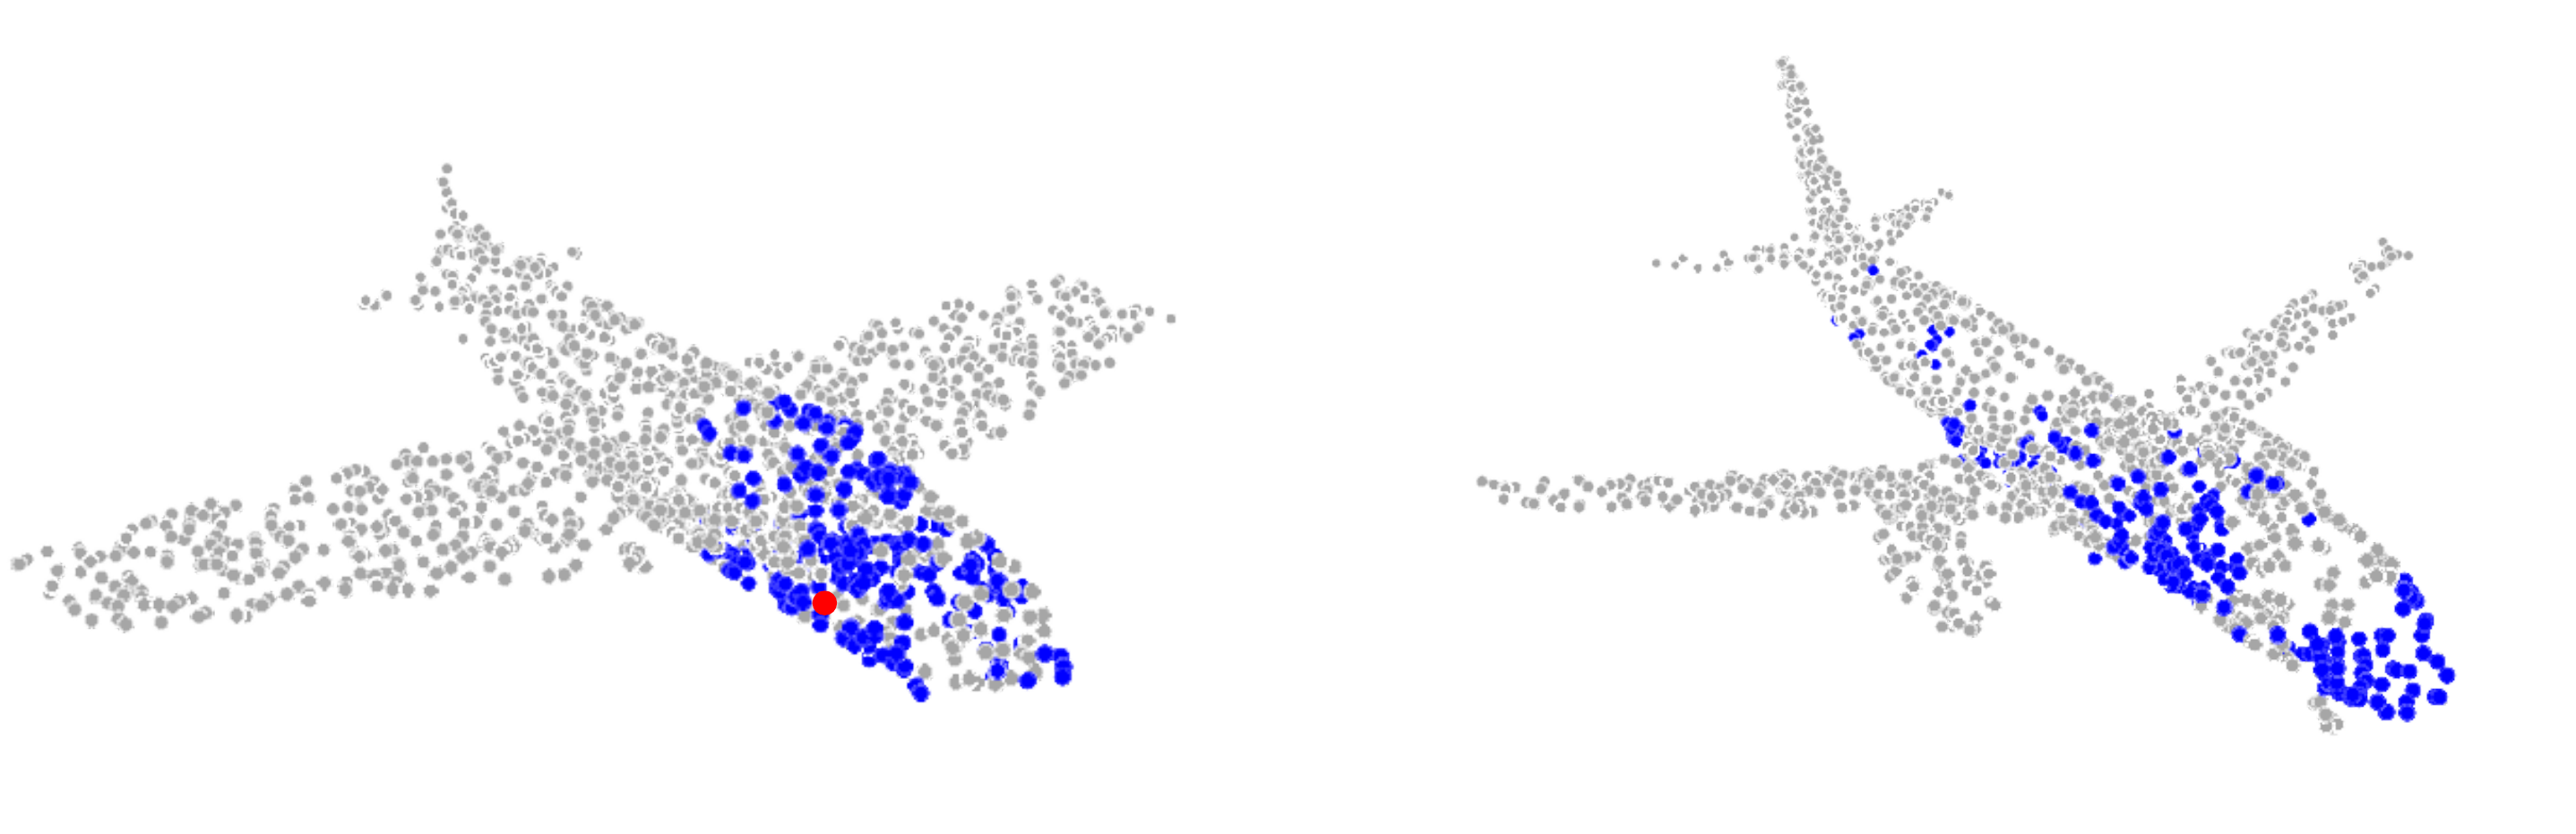}
    \caption{Illustration of zero-shot correspondence learning.}
    \label{fig:feat-vis-v2}
\end{figure}
