# Supplementary material for: 3D Feature Prediction for Masked-AutoEncoder-Based Point Cloud Pretraining
Source: arXiv:2304.06911 source file (2024-04-28)
Supplement: Supplementary file 4 [file supp-fig-feat-vis.tex]

\begin{figure*}
    \centering
    \begin{overpic}[width=0.8\linewidth]{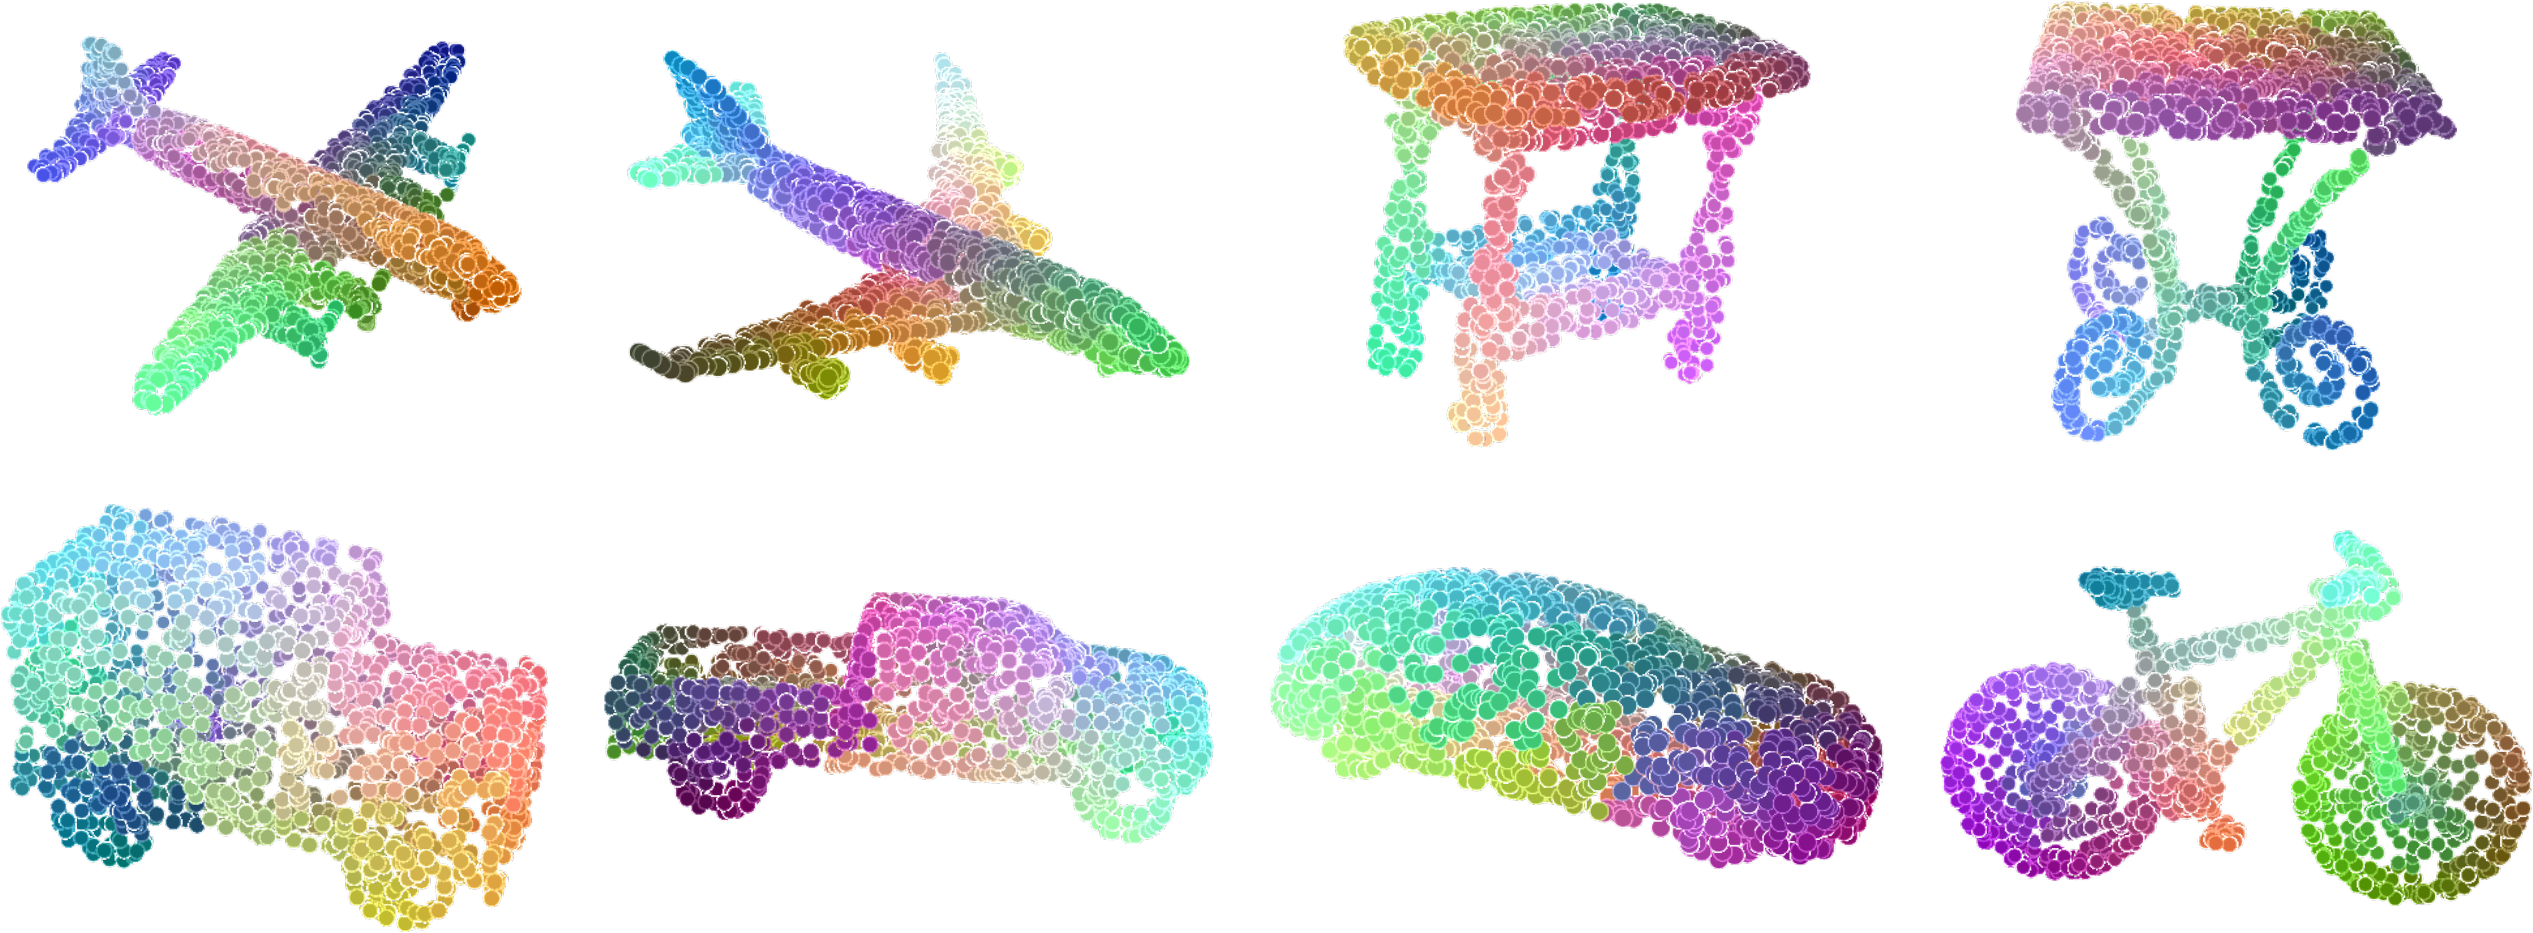}
    \end{overpic}
    \caption{\textbf{Feature visualization results of our method.} The color difference between different points characterizes their feature differences.} 
    \label{fig:supp-feavis} %\vspace{-4mm}
\end{figure*}
