# Supplementary material for: 3D Feature Prediction for Masked-AutoEncoder-Based Point Cloud Pretraining
Source: arXiv:2304.06911 source file (2024-04-28)
Supplement: Supplementary file 8 [file supp_modelnet.tex]

\begin{table*}[t]
\small
\begin{minipage}[b]{.45\linewidth}
    \centering
   \setlength\tabcolsep{5pt}% 调整列间距
    \begin{tabular}{lc}
        \toprule
        \textbf{Method} & \textbf{ModelNet40} \\
        \midrule
        PointViT$^{\dagger}$ ~\cite{Yu_2022_CVPR}     & 91.4 \\
        PointBERT~\cite{Yu_2022_CVPR}    & 93.2 \\
        MaskDiscr~\cite{Liu2022maskdis}  & 93.8 \\
        MaskSurfel~\cite{zhang2022masked} & 93.6 \\
        PointMAE~\cite{Pang2022MaskedAF} & 93.8 \\
        \rowcolor{gray!20}MaskFeat3D (PointViT)    & \textbf{93.9} \\
        \bottomrule
    \end{tabular}
    \captionof{table}{\small{\textbf{Shape classification fine-tuned on ModelNet40.} All the methods use the same transformer backbone architecture. $^{\dagger}$ represents the \textit{from scratch} results and all other methods represent the \textit{fine-tuning} results using pretrained weights.}}
    \label{tab:modelnet40}
\end{minipage}\hspace{.02\linewidth}
\begin{minipage}[b]{.5\linewidth}
 \setlength\tabcolsep{5pt}
    \begin{tabular}{lc}
        \toprule
        \textbf{Method} & \textbf{Acc. (\%)} \\
        \midrule
        %Random &  60.2\% \\
        3D-GAN~\cite{wu2016learning}  & 83.3 \\
        Latent-GAN~\cite{achlioptas2018learning} & 85.7 \\
        SO-Net~\cite{li2018so} & 87.3 \\
        MAP-VAE~\cite{han2019multi} & 88.4 \\
        Jigsaw~\cite{sauder2019self} & 84.1 \\
        FoldingNet~\cite{yang2018foldingnet} & 88.4 \\
        DGCNN + OcCo~\cite{wang2021unsupervised} & 89.7 \\
        DGCNN + STRL~\cite{huang2021spatio} & 90.9 \\
        \midrule 
        PointViT + OcCo$^*$~\cite{wang2021unsupervised} & 89.6 \\
        PointBERT~\cite{Yu_2022_CVPR}$^*$ & 87.4 \\
        %MaskDiscr$^*$ & \\
        PointMAE~\cite{Pang2022MaskedAF}$^*$ & 88.5 \\
        \rowcolor{gray!20}MaskFeat3D (PointViT) $^*$ & \textbf{91.1}\\
        
        \bottomrule
    \end{tabular}
    \captionof{table}{\small{\textbf{Linear evaluation for shape classification on ModelNet40}. This task is sensitive to the encoder backbone. Different * methods use the same Transformer encoder backbone.}}
    \label{tab:svm}
\end{minipage}
\end{table*}
